# Supplementary material for: In-Context Matting
Source: arXiv:2403.15789 source file (2024-03-23)
Supplement: Supplementary file 1 [file data_supp.pdf]

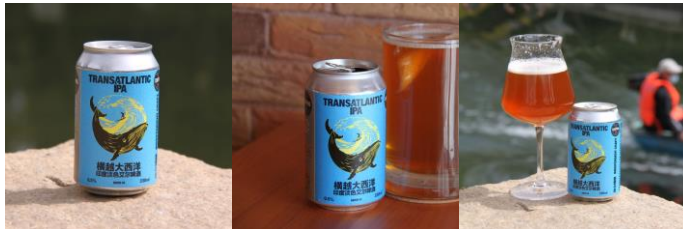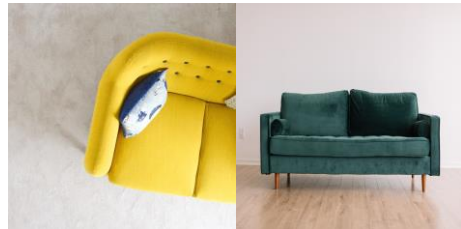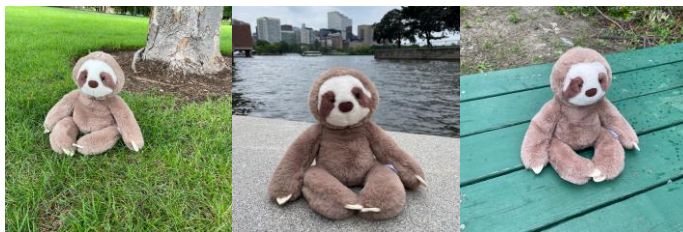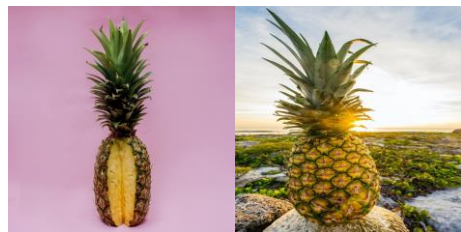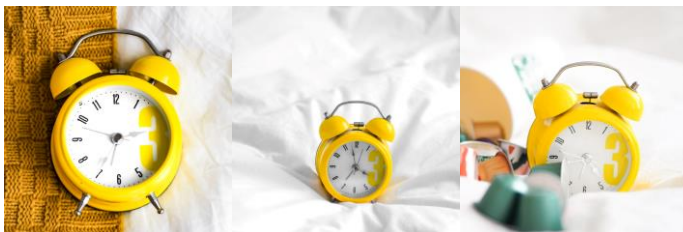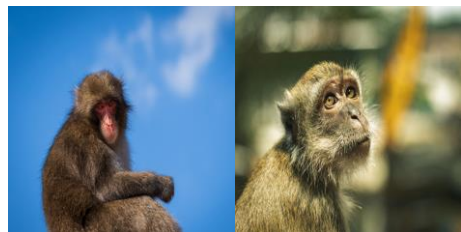

(a) Same instance

(b) Same category

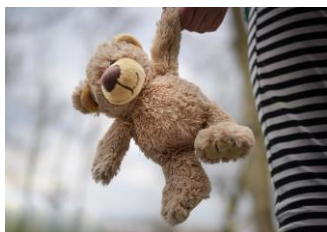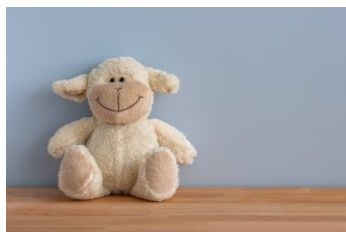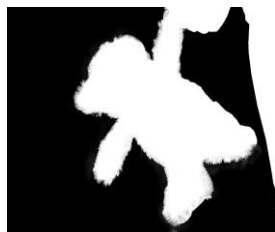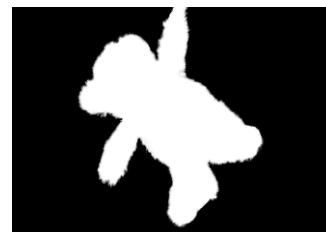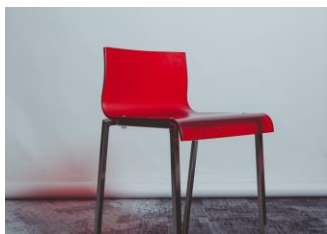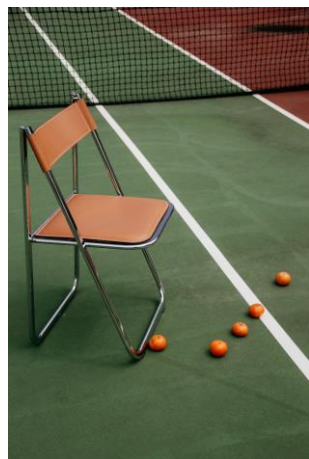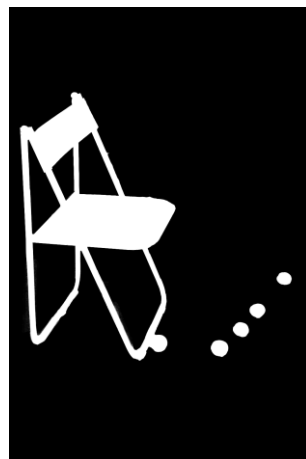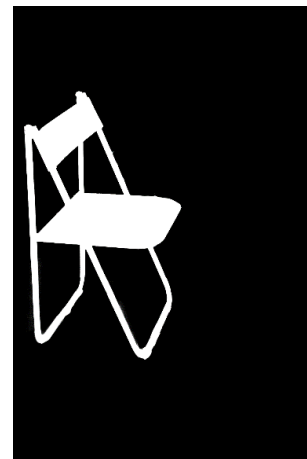

Reference

Image

AIM-500

ICM-57
